# Supplementary material for: Post-Processing of High-Dimensional Data
Source: arXiv:1906.05669 source file (2019-09-23)
Supplement: Supplementary file 1 [file appendix.tex]

% !TEX root = ../14_tensor_post-proc.tex
% !TEX encoding = UTF-8 Unicode
% RCSID:       $Id: appendix.tex,v 1.4 2019/05/27 23:28:20 hgm Exp $
% Author:      Hermann G. Matthies
% Contact:     wire@tu-bs.de
% =================================

%% texfile{
%%  AUTHOR    = "$Author: hgm $",
%%  VERSION   = "$Revision: 1.4 $",
%%  DATE      = "$Date: 2019/05/27 23:28:20 $",
%%  FILENAME  = "$RCSfile: appendix.tex,v $"}

\section*{Appendix}
All's well that ends well.  ...
\vspace{1cm}
\subsection*{Notation} \label{SS:notation}
\paragraph{Variables and Constants:}
In general variables should be written in a slanted or italic font, like
\[ \alpha, \delta, \xi, \vphi, \Delta, \Phi, \Omega, a, d, x, f, D, F, \]
and constants with an upright font, like
\[ \upgamma=0.57721\dots, \uppi = 3.14159265\dots, \upvarphi = 1.61803\dots, 
   \ee=2.71828\dots, \ii=\sqrt{-1}.
\]

\paragraph{Operators and fixed Objects:}
Also operators should be upright like differential, derivatives, etc.   
\[
  \di \omega, \; \frac{\di f}{\di x},\; \Di F, \;\int_{\C{X}} f(x)\, \di x,\quad\upDelta = \nabla^2.
\]
Also named objects like the Kronecker-$\updelta$ --- $\updelta_{i j}$ ---
 and Dirac's $\updelta$ --- $\int_{\D{R}} \updelta_{a}(x)\,f(x)\, \di x = f(a)$
in an upright font.

\paragraph{Householder Convention:}
Additionally, when dealing with linear spaces, use the \emph{Housholder}
convention --- unless usual convention demands otherwise:
\begin{description}
\item[Scalars] with small slanted Greek letters
         \[ \alpha, \beta, \gamma, \delta, \dots \]
\item[Sets of scalars] with capital slanted Greek letters
         \[ \Gamma, \Delta, \Phi, \Xi, \Omega, \dots \]
\item[Vectors] of general spaces with small (serif) italic Latin letters
         \[ a, u, v, w, x, y, z, \dots \]       
\item[Linear Operators] of general spaces with capital (serif) italic Latin letters
         \[ A, U, V, F, X, Y, Z, \dots \]
\item[Vectors with components] as elements of $\D{R}^n$ or $\D{C}^n$ with
     \tbf{bold}  small italic (serif) Latin or Greek letters, and their components with the
     corresponding non-bold letter
  \[ \vek{\alpha} = [\alpha_1,\alpha_2,\dots,\alpha_n]^\trpos,\, 
     \vek{u} = [u_1,\dots,u_n]^\trpos,\, 
     \vek{\xi} = [\xi_1,\dots,\xi_n]^\trpos,\, 
     \vek{x} = [x_1,\dots,x_n]^\trpos,\, \dots \]  
\item[Matrices] with \tbf{bold} capital italic (serif) Latin or Greek letters,
     and their components with the
     corresponding non-bold letter
  \[ \vek{A} = [A_{11},A_{12},\dots,A_{nn}],\, \vek{\Xi} = [\Xi_{11},\Xi_{12},\dots,\Xi_{nn}],\, 
     \vek{X} = [X_{11},X_{12},\dots,X_{nn}],\, \dots \]  
\end{description}
         
\paragraph{Additional Conventions:}      
\begin{description}
\item[Multi-Indices]  as elements of $\D{N}^n$ or $\D{N}_0^n$  with
     \tbf{bold}  small italic Latin letters, and their components with the
     corresponding non-bold letter
  \[ \vek{m} = (m_1,m_2,\dots,m_n],\, \vek{\ell} = [\ell_1,\ell_2,\dots,\ell_n], \dots \] 
  or ?
\item[Multi-Indices]  as elements of $\D{N}^n$ or $\D{N}_0^n$  with
     \tbf{bold} small Fraktur letters, and their components with the
     corresponding non-bold Latin letter
  \[ \F{m} = (m_1,m_2,\dots,m_n],\, \F{k} = [k_1,k_2,\dots,k_n], \dots \] 
\item[Linear Spaces] and their subsets with capital calligraphic Latin letters
         \[ \C{A}, \C{U}, \C{V}, \C{F}, \C{X}, \C{Y}, \C{Z}, \dots \]       
\item[Spaces of Linear Operators] with capital script Latin letters
         \[ \E{L}(\C{U}),\; \E{L}(\C{X},\C{Y}), \dots \]
\item[Sets of Sets] like topologies and $\sigma$-algebras with capital Fraktur letters
        \[ \F{G}, \; \F{T}, \; \F{A}, \dots \]
\item[Tensors] as elements of e.g.\ $\D{R}^{n_1\times n_2 \times \dots \times n_d}$
   with slanted sans-serif \tbf{bold} letters, and their components with the
   corresponding slanted sans-serif non-bold letters
   \[ \tnb{w}=(\tns{w}_{i_1,\dots,i_d}),\;  \tnb{M}= (\tns{M}_{a b c d}),\;
    \tnb{y}=(\tns{y}_{{i_1}{k_1}i_2 k_2}),\; \tnb{\beta}=(\tns{\beta}_{i_1,\dots,i_\ell}),\;
    \tnb{\Theta}=(\tns{\Theta}_{\ell_1,\dots,\ell_d})
     \dots \]
       or in Penrose's \emph{symbolic} index notation
      with slanted sans-serif or serif non-bold letters
   \[ \tensor{\tns{M}}{^a_b^{cd}_e},\; \tensor[^a_b^c_d]{\tns{A}}{^a_b^c_d},\;
   \tensor{R}{_i^j_k},\; \tensor{\Gamma}{^i_j_k},\; 
   \tensor{\tns{\Omega}}{^i_\ell^k_m_n},   \dots \]
\end{description}

\subsection*{Tensor package} \label{SS:tensors}
\[ M\indices{^a_b^{cd}_e} = \tensor{M}{^a_b^{cd}_e}\]
\begin{verbatim}
M\indices{^a_b^{cd}_e} = \tensor{M}{^a_b^{cd}_e}
\end{verbatim}

\[ \tensor[^a_b^c_d]{M}{^a_b^c_d} \neq \tensor*[^a_b^c_d]{M}{^a_b^c_d} \]
\begin{verbatim}
 \tensor[^a_b^c_d]{M}{^a_b^c_d} \neq \tensor*[^a_b^c_d]{M}{^a_b^c_d}
\end{verbatim}

\[ \tensor*{M}{*^{i_1}_{m_1}^{i_2}_{m_2}^{i_3}_{m_3}^{i_4}_{m_4}} =
   M\indices*{*^{i_1}_{m_1}^{i_2}_{m_2}^{i_3}_{m_3}^{i_4}_{m_4}} \]
\begin{verbatim}
\tensor*{M}{*^{i_1}_{m_1}^{i_2}_{m_2}^{i_3}_{m_3}^{i_4}_{m_4}}=
  M\indices*{*^{i_1}_{m_1}^{i_2}_{m_2}^{i_3}_{m_3}^{i_4}_{m_4}}
\end{verbatim}

\[ \tensor{M}{^a_b^c_d} \]
\begin{verbatim}
\renewcommand\indexmarker{\cdot}   \tensor{M}{^a_b^c_d}
\end{verbatim}

\[ \nuclide[14][6]{C} \quad \text{and} \quad \nuclide[4][2]{\upalpha} \]
\begin{verbatim}
\nuclide[14][6]{C} \quad \text{and} \quad \nuclide[4][2]{\upalpha} 
\end{verbatim}

\subsection*{Test of math fonts} \label{SS:testf}
\paragraph{Slanted:} --- serifs
\[ a, \alpha, A, \Phi, \phi, \vphi, \qquad 
     \vek{a}, \vek{\alpha}, \vek{A}, \vek{\Phi}, \vek{\phi}, \vek{\vphi} \]

\paragraph{Slanted:} --- sans serif
\[ \tns{a}, \tns{\alpha}, \tns{A}, \tns{\Phi}, \tns{\phi}, \tns{\vphi}, \qquad
  \tnb{a}, \tnb{\alpha}, \tnb{A}, \tnb{\Phi}, \tnb{\phi}, \tnb{\vphi} \]
   
\paragraph{Other:}  --- no small letters
\[ \C{E}, \C{Q}, \C{R}; \D{E}, \D{Q}, \D{R}; \E{E}, \E{Q}, \E{R}\]

\paragraph{Fraktur:}
\[ \F{e}, \F{q}, \F{r}; \F{E}, \F{Q}, \F{R} \]

\paragraph{Upright:} --- serifs and sans-serif, no small greek letters
\[ \mrm{a}, \mrm{A}, \mrm{\Phi},\qquad \mat{a}, \mat{A}, \mat{\Phi}, \qquad 
 \ops{a}, \ops{A}, \ops{\Phi},\qquad \opb{a}, \opb{A}, \opb{\Phi} \]

\paragraph{Small Greek upright}
\[ \upalpha, \uppi, \upgamma, \upphi, \upvarphi, \uppsi, \upxi, \upeta, \upzeta \]

%  $Log: appendix.tex,v $
%  Revision 1.4  2019/05/27 23:28:20  hgm
%  tiny correction
%
%  Revision 1.3  2019/04/13 18:43:03  hgm
%  describes notation
%
%  Revision 1.2  2019/04/13 10:30:57  hgm
%  little changes, shifted fonts
%
%  Revision 1.1  2019/03/08 23:24:43  hgm
%  initial check-in
%
%
%
%
%

%%% Local Variables: 
%%% mode: latex
%%% TeX-master: "../14_tensor_post-proc"
%%% End: 
